# Supplementary material for: INDIGO: Page Migration for Hardware Memory Disaggregation Across a Network
Source: arXiv:2503.18140 source file (2025-03-23)
Supplement: Supplementary file 1 [file appendix.tex]

\section{Appendix}

\subsection{Network Cost Model for Page Migration}
\label{ss:network_cost_model_derivaton}

We derive the network cost model for swapping two pages \textbf{p} and \textbf{d} for a time interval $\Delta T$.
Page \textbf{p} (the promoted page) is initially located in the remote memory pool and is swapped into local memory.
On the other hand, Page \textbf{d} (the demoted page) is initially located in local memory and is swapped into the remote memory pool to take the place of Page \textbf{p}.
We consider the following cost/benefit associated with the swap:
\begin{enumerate*}[label=(\alph*)]
    \item \textit{Access locality benefit} for page \textbf{p},
    \item \textit{Access locality cost} for page \textbf{d},
    \item \textit{Network transfer cost} of the swap, and
    \item \textit{Computational overhead} of the swap.
\end{enumerate*}

\noindent \emph{Access Locality Benefit/Cost: } All accesses to the page \textbf{p} are directed to local memory instead of the remote memory pool.
Therefore, total memory access time reduction (locality benefit) is the number of accesses multiplied by the reduction in latency:
\begin{align*}
    \text{Locality Benefit} = \#\text{access}_p \times (\text{remote latency} - \text{local latency})
\label{eq:locality_benefit}
\end{align*}
where $\text{access}_p$ is the number of times page \textbf{p} is accessed and $(\text{remote latency} - \text{local latency})$ (i.e. $\Delta \text{latency}$) is the difference between latency of the local node and remote memory pool. Similarly, there is a loss of locality associated with demoted page \textbf{d}.
\begin{align*}
    \text{Locality Cost} = \#\text{access}_d \times (\text{remote latency} - \text{local latency})
\end{align*}

\noindent \emph{Network Transfer Cost: } The network transfer cost is associated with migrating the two pages from remote to local memory (and vice versa).
As pages are typically large (in the order of several KBs), transmission delay dominates the total network transfer cost.
\begin{align*}
    \text{Network Cost} = \frac{\text{page size}}{\text{available bandwidth}}
\end{align*}

\noindent \emph{Computational Cost: } Computational cost is associated with the bookkeeping overhead of page migration that includes handling interrupts, remapping of page table entries, flushing of the translation lookaside buffer (TLB), and so on.
We consider this cost as a constant in the model.\\

\noindent \emph{Inequality Derivation: } By equating the total benefit to be greater than the total cost, we derive:

\begin{align*}
    \text{Locality Benefit} \geq \text{Locality Cost} + \text{Network Cost} +\text{Comp Cost}\\
    (\#\text{access}_p -\#\text{access}_d) \times \Delta \text{latency} \geq
    \frac{\text{page size}}{\text{available bandwidth}} \\ + \text{Comp Cost}
\end{align*}

As most page migration mechanisms measure access rate, we substitute the number of accesses ($\#\text{access}_p$) with the access rate ($\text{access}_p$) over an interval $\Delta T$.
$\Delta T$ represents the time window between the current and the next swap which would depend on the specific page migration mechanism implementation.

\begin{align*}
    \int_{0}^{\Delta T}(\text{access}_p -\text{access}_d) dt \times \Delta \text{latency} \geq
    \frac{\text{page size}}{\text{available bandwidth}} \\+  \text{Comp Cost}
\end{align*}

By rearranging the equation terms, we derive the model mentioned in Equation~\cref{eq:axiom_page_migration}.

\subsection{Bipartite Matching Formulation for Optimal Page Promotion}
\label{ss:bipartite_matching}

\begin{figure}[ht]
    \includegraphics{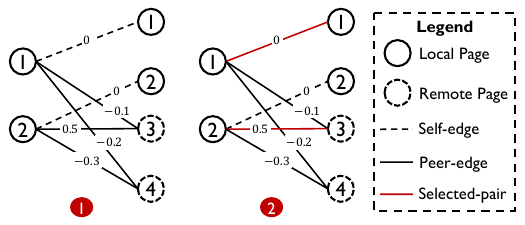}
    \caption{Page promotion optimization solved with bipartite matching. (1) The bipartite graph $G_p$ for page promotion; (2) Possible solution to the bipartite matching: Highlighted edges as the page promotion configuration. Edge weights are for illustrative purposes only.}
    \label{fig:bipartie_matching}
\end{figure}
Our goal is to solve the optimization problem for deciding which pair of pages should be swapped, assuming the network cost model presented in Equation~\cref{eq:axiom_page_migration}.
We are given a set of local pages $\mathcal{P}$, and a set of remote pages $\mathcal{D}$, 
at each decision time step, we would like to decide on a subset of 
pages $\mathbf{p} \subseteq \mathcal{P}$ to be swapped with a subset of pages $\mathbf{d} \subseteq \mathcal{D}$, while maximizing the sum of benefit (equivalent to minimizing network cost) of swapping by rearranging~\cref{eq:axiom_page_migration}.
This can be formally represented as:
\begin{align*}
    P: &\max \: \sum_{p \sim \mathbf{p}, d \sim \mathbf{d}}\text{NetBenefit}(p, d, \Delta t) \\
    & \mathbf{s.t.}\:\:\:\:|\mathbf{p}| = |\mathbf{d}|
\end{align*}
where \begin{align*}
    \text{NetBenefit}(p,d,\Delta t) = \int_{0}^{\Delta T} (\text{access}_p - \text{access}_d) \: dt  \\
     \:\: - \frac{\text{page size}}{\text{bandwidth} \times \Delta \: \text{latency}} - k
\end{align*}

\noindent \textbf{Constructing the Bipartite Graph.}
$P$ can be effectively solved as a maximum weight bipartite-matching problem, in which the solution to the problem, $M$, 
indicates the set of pages to swap at each decision time step such that the total benefit is maximized. The bipartite graph $G_p(V, E)$ is constructed as follows: 
\begin{enumerate}
    \item Let $V_{localpages} = \mathcal{D}, V_{remotepages} = \mathcal{P}, V_{allpages} = \mathcal{D \cup P}$, and $V = V_{localpages} + V_{allpages}$. $V_{localpages}$ and $V_{allpages}$ are disjoint bipartite of the $G_p$
    \item For all pair of vertices $(v_{localpage},v_{page}) \in V_{localpages} \times V_{allpages}$, we construct an edge $e \in E$ that connects the subgraph $V_{localpages}$ and $V_{allpages}$ if and only if 
    \begin{enumerate}
        \item $v_{localpage} == v_{page}$, i.e., the page is paired to itself.
        \item $v_{localpage} \neq v_{pages}$ i.e., the two pages have different localities (local vs. remote).
    \end{enumerate}
    $v_{localpage}$ and $v_{page}$ are not a potential swapping pair if $v_{localpage} \neq v_{page}$ but their locality are the same.
    \item For all edges $e \in E$, we assign edge weight $w$ as follows:
    \begin{enumerate}
        \item if $v_{localpage} == v_{page}$, then $w = 0$.
        \item else, $w = \text{NetBenefit}(v_t = p, v_{t+\Delta t} = d, \Delta t)$.
    \end{enumerate}
To summarize, we assign a positive weight to an edge if and only if two pages can be swapped (i.e. they have different locality) and such swapping results in a net positive benefit.
\end{enumerate}
We can now solve $G_p$ as a bipartite problem by finding the matching edges $M \subset E$.
The pages that are paired to themselves mean a no-op and hence we assigned zero benefits.
The solution $M$ can be found in $O(|V|^3)$ time using the Hungarian Maximum Weight Matching algorithm~\cite{kuhn1955}.
